# Supplementary material for: Parametric generation of spin waves in nano-scaled magnonic conduits
Source: arXiv:2106.10727 ancillary file (2022-01-15)
Supplement: Supplementary file 1 [file Supplement.pdf]

# Supplemental material
# -
# Parametric generation of spin waves in nano-scaled magnonic conduits


Björn Heinz,[1,*] Morteza Mohseni,[1] Akira Lentfert,[1] Roman Verba,[2] Michael Schneider,[1] Bert Lägel,[3] Khrystyna Levchenko,[4] Thomas Brächer,[1] Carsten Dubs,[5] Andrii V. Chumak,[4] and Philipp Pirro[1]

[1] *Fachbereich Physik and Landesforschungszentrum OPTIMAS, Technische Universität Kaiserslautern, D-67663 Kaiserslautern, Germany*
[2] *Institute of Magnetism, UKR-03142 Kyiv, Ukraine*
[3] *Nano Structuring Center, Technische Universität Kaiserslautern, D-67663 Kaiserslautern, Germany*
[4] *Faculty of Physics, University of Vienna, A-1090 Wien, Austria*
[5] *INNOVENT e.V. Technologieentwicklung, D-07745 Jena, Germany*


## CONTENTS


I. Theoretical calculation of the spin-wave dispersion 1

II. Micro-magnetic simulation of the spin-wave dispersion 3

III. Fourier spectrum of the pumping pulse 3

IV. Micro-magnetic simulations of the pumping process 3

V. Associated power law of the experimentally observed pumping process 5

VI. Extraction of the effective spin-wave relaxation time 5

References 6


## I. THEORETICAL CALCULATION OF THE SPIN-WAVE DISPERSION

Figure S1 shows theoretical calculations of the spin wave dispersion and connected parameters [1], the ellipticity coefficient, the coupling parameter, intrinsic and radiative threshold respectively and the complete threshold [2] for a fixed frequency of 3.5 GHz. The parameters of the plain film, extracted by VNA-FMR and micro-focused BLS spectroscopy as stated in the manuscript, have been assumed for the calculations, with the exception of a saturation magnetization of $M_\mathrm{s}$ =125 kA m$^{-1}$ for the 100 nm-wide conduit, chosen to fit the spin-wave dispersion to the observed pump spectrum. The reduced magnetization can be attributed to the influence of microwave and laser heating, while an influence of the structuring process cannot be excluded either. Please note, the calculations are performed according to Eq. S1, including the partial pinning of the spin-wave width mode profile for the 1000 nm-wide conduit and the effective unpinning of the profile for the 100 nm-wide conduit [1]:

$$\omega_\mathrm{k} = \sqrt{\left(\omega_\mathrm{H} + (\lambda^2 K^2 + F^{\mathrm{zz}}_{k_\mathrm{x}})\omega_\mathrm{M}\right) \times \left(\omega_\mathrm{H} + (\lambda^2 K^2 + F^{\mathrm{yy}}_{k_\mathrm{x}})\omega_\mathrm{M}\right)}. \tag{S1}$$

Here, $\omega_\mathrm{k}$ is the spin-wave frequency, $\omega_\mathrm{H} = \gamma B_\mathrm{ext} = \gamma\mu_0 H_\mathrm{ext}$ due to a negligible demagnetization along the conduit, $\omega_\mathrm{M} = \gamma\mu_0 M_\mathrm{s}$ and $\lambda = \sqrt{\frac{2A_\mathrm{ex}}{\mu_0 M_\mathrm{s}^2}}$. Moreover, $K^2 = k_\mathrm{x}^2 + k_\mathrm{y}^2$ is the total wavevector and $F^{\mathrm{zz}}_{k_\mathrm{x}}$ and $F^{\mathrm{yy}}_{k_\mathrm{x}}$ denote the dynamic demagnetization tensor components out-of-plane and in-plane perpendicular to the waveguide.


* bheinz@rhrk.uni-kl.de

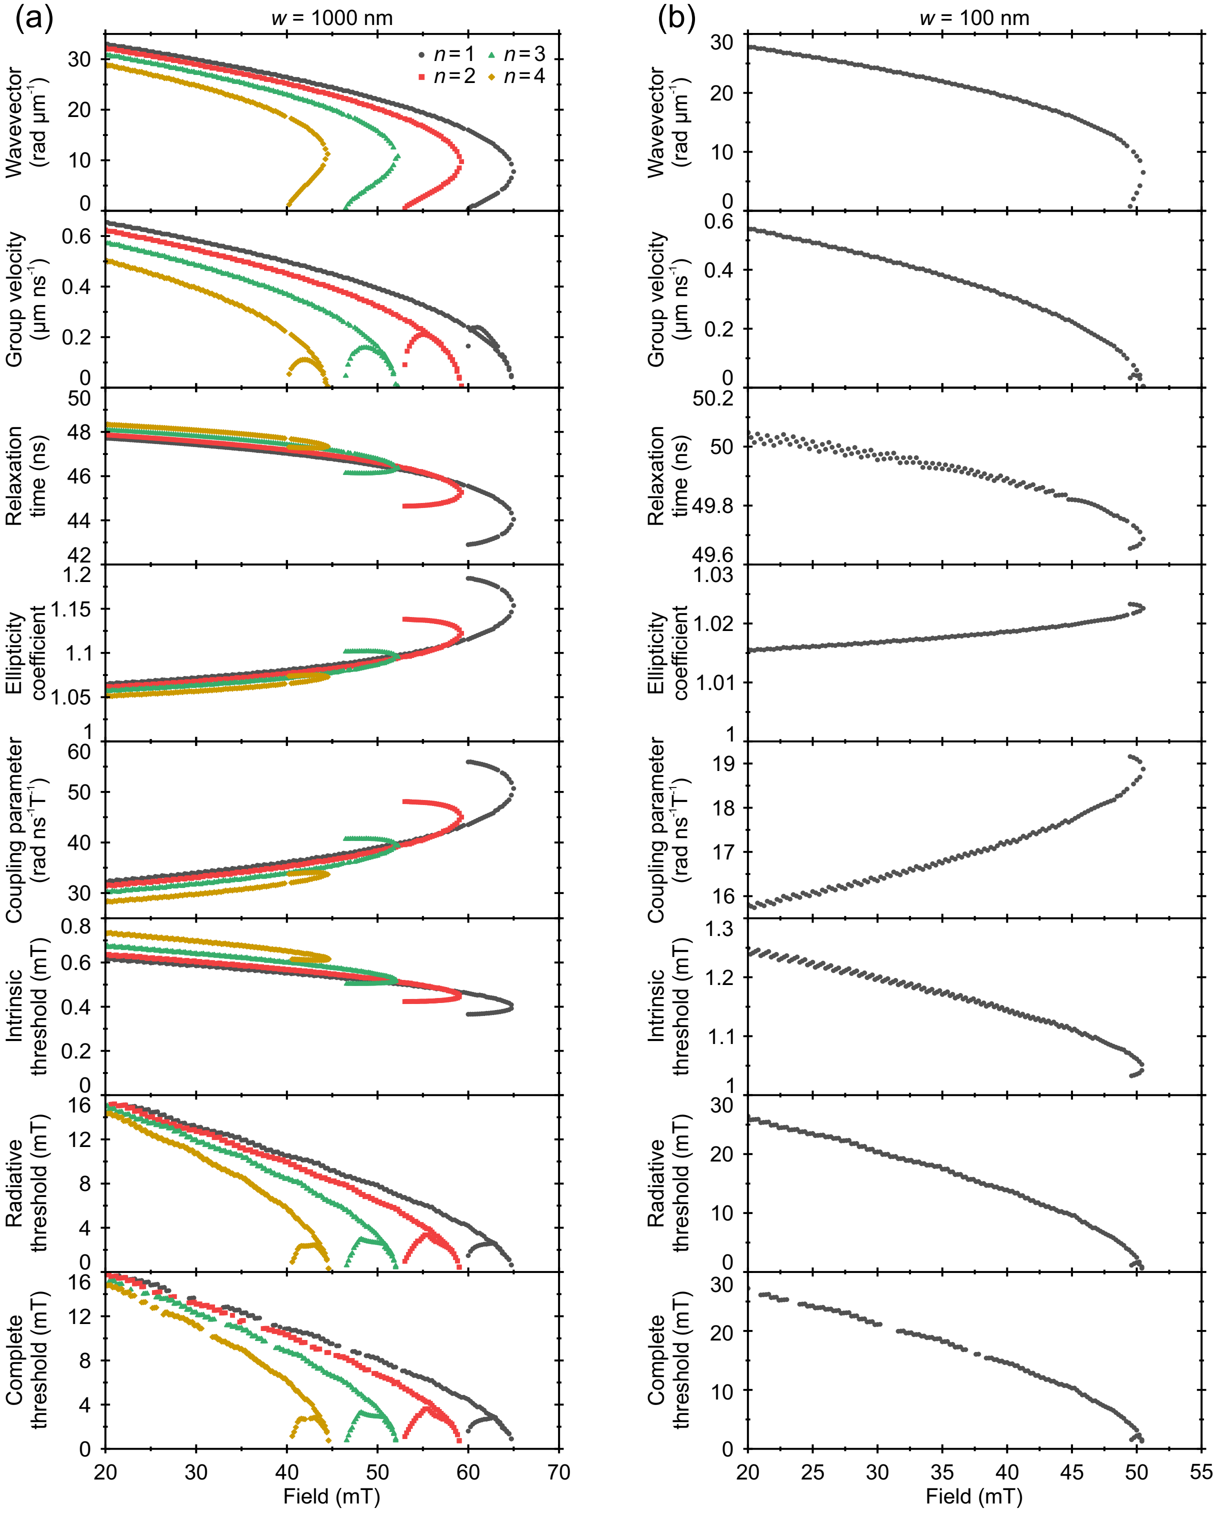


FIG. S1. Theoretical calculations of the spin-wave dispersion, connected parameters, the ellipticity coefficient, the coupling parameter,intrinsic and radiative threshold respectively and the complete threshold for a fixed frequency of 3.5 GHz for (a) $w = 1000$ nm and (b) $w = 100$ nm. A reduced effective magnetization of $M_s$ =125 kA m$^{-1}$ has been assumed for the 100 nm-wide conduit.

## II. MICRO-MAGNETIC SIMULATION OF THE SPIN-WAVE DISPERSION

In Fig. S2(a), a micro-magnetic simulation of the dispersion relation for the 100 nm-wide conduit is shown. The simulation has been carried out using the MuMax3 framework [3] for $\mu_0 H_{\mathrm{ext}} = 50\,\mathrm{mT}$ and assuming the parameters of the plain film, but taking the reduced effective magnetization into account. The fundamental width mode $n = 1$, as well as the first higher-order width mode $n = 2$ are shown, exhibiting a large frequency gap in between, which is caused by the strong quantization and the increased impact of the exchange interaction for the $n = 2$ mode. Thus, the 100 nm-wide conduit effectively resembles a single-mode system within the limits of the experiment. A trust check can be made, comparing the simulation and the theoretical calculation for the fundamental mode, which is shown in Fig. S2(b). A perfect agreement within the frequency uncertainty of the simulation is found.

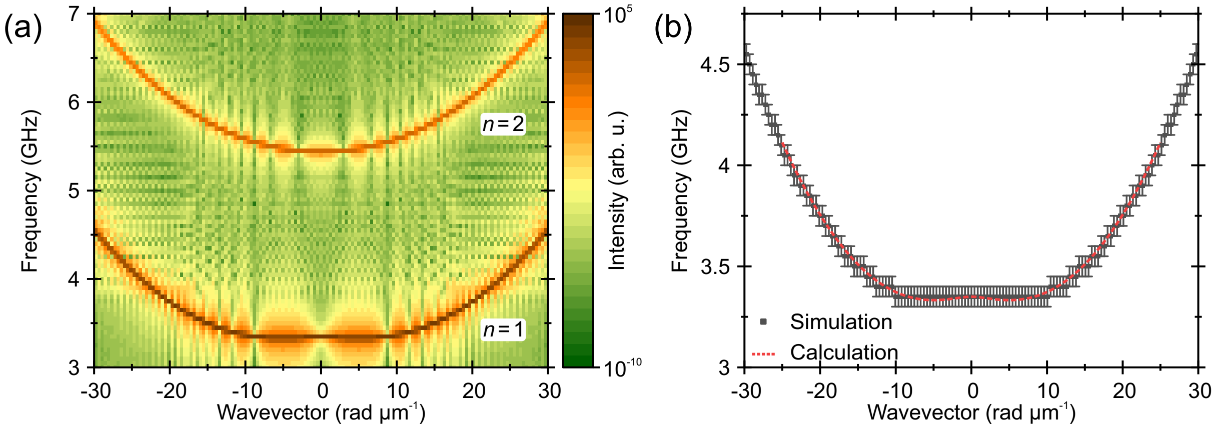


FIG. S2. (a) Simulated dispersion relation of the 100 nm-wide conduit for $\mu_0 H_{\mathrm{ext}} = 50\,\mathrm{mT}$. Intensity displayed in log-scale. (b) Comparison of the simulated fundamental mode's dispersion relation and the theoretical calculation of Fig. S1(b).

## III. FOURIER SPECTRUM OF THE PUMPING PULSE

Parametric excitation by parallel pumping can be carried out either using a pumping field which is continuous in time or of finite duration by applying it in a pulsed manner as it is done in the manuscript. We would like to point out, that utilizing finite pulses allows for resonant processes to occur within the frequency uncertainty of the pumping pulse, which is given by the Fourier transformation of the pulse's time trace. However, as it can be seen from Fig. S3, the influence of this effect is expected to be on the order of $\pm 50\,\mathrm{MHz}$, which is much smaller than the frequency shift observed in the experiment.

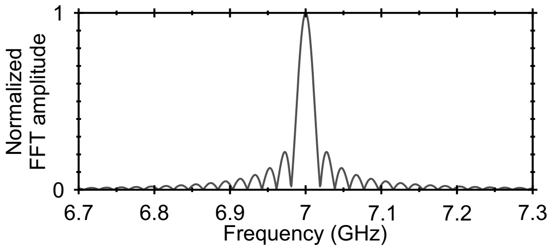


FIG. S3. Normalized Fourier transformation of the pumping pulse time trace. Carrier frequency 7 GHz and pulse length 50 ns with rising/falling edges of each 5 ns assuming an exponential slope.

## IV. MICRO-MAGNETIC SIMULATIONS OF THE PUMPING PROCESS

To classify the experimental observations, we perform micro-magnetic simulations of the pumping process using the MuMax3 open-source framework [3]. The 100 nm-wide conduit is modeled with a rectangular cross-section and

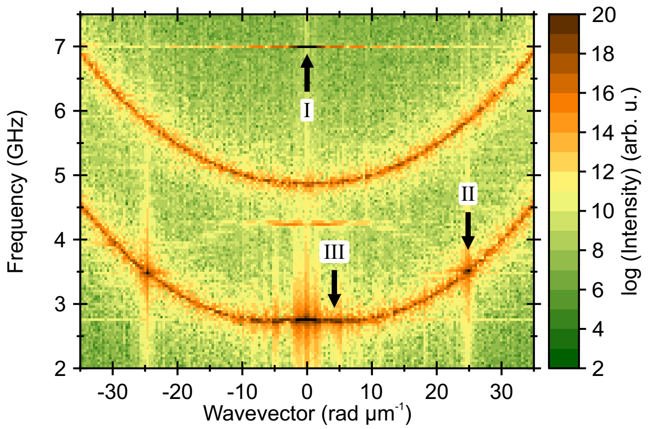


FIG. S4. Simulated spin-wave dispersion of the 100 nm-wide conduit taking in-plane and out-of-plane components of the pumping field into account. A directly driven forced oscillation (I) at 7 GHz, parallel pumping (II) at half the pumping frequency $f_\mathrm{p}/2 = 3.5\,\mathrm{GHz}$ and an additional spin-wave population (III) in the dipolar regime of the dispersion at 2.76 GHz are observed. Applied pumping ac-current amplitude 100 mA, magnetic field $\mu_0 H_\mathrm{ext} = 30\,\mathrm{mT}$.

assuming the plain film parameters as stated above, but taking a reduce effective magnetization of $M_\mathrm{s}$ =125 kA m$^{-1}$ into account to match the pump spectrum. In contrast to the theoretical calculations, the pumping field is included using its real spatial distribution, thus, not only the pumping field's in-plane component $h_\mathrm{p}^\mathrm{x}$ parallel to the conduit is considered but also the out-of-plane component $h_\mathrm{p}^\mathrm{z}$ perpendicular to the internal magnetization. In Fig. S4, an exemplary simulated spin-wave dispersion for an applied ac-current amlitude of 100 mA and $\mu_0 H_\mathrm{ext} = 30\,\mathrm{mT}$ is shown, where several peaks are observed within the spectrum: (I) a directly driven forced oscillation at 7 GHz, caused by the out-of-plane component of the pumping field, (II) parallel pumping at half the pumping frequency $f_\mathrm{p}/2 = 3.5\,\mathrm{GHz}$ as predicted by the theory and (III) an additional spin-wave population in the dipolar regime of the dispersion at 2.76 GHz. A power (current) dependent investigation is performed, shown in Fig. S5(a), and the amplitude of the respective signals is extracted in dependency of the applied ac-current amplitude. While the directly driven forced oscillation is observed for all powers, the onset of the resonant PP process is found for large powers at half the pumping frequency $f_\mathrm{p}/2 = 3.5\,\mathrm{GHz}$ as predicted by the theory. Surprisingly, the additional spin-wave population at 2.76 GHz is already present for minimal applied powers and does not possess a threshold. A linear approximation (using a double logarithmic plot) reveals that the associated power law ($Intensity \propto Power^m$) is of 1$^\mathrm{st}$-order ($m = 1.001$), which is a strong indication of a directly driven linear excitation. In Fig. S5(b) the simulation is repeated but taking

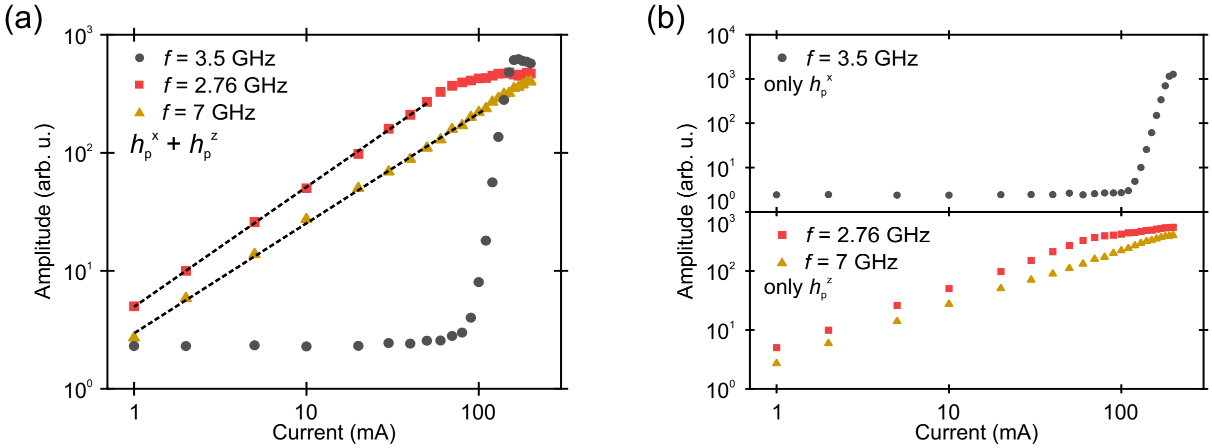


FIG. S5. Power dependent simulation series of the 100 nm-wide conduit for $\mu_0 H_\mathrm{ext} = 30\,\mathrm{mT}$. (a) Taking in-plane $h_\mathrm{p}^\mathrm{x}$ and out-of-plane $h_\mathrm{p}^\mathrm{z}$ pumping field components into account reveals an onset of PP at 3.5 GHz for large powers, the presence of a forced excitation at 7 GHz and an additional excitation at 2.76 GHz, which does not possess a threshold. A linear approximation (dashed black line) reveals an intensity-power correlation with a 1$^\mathrm{st}$-order power law. (b) Taking only the in-plane component (top panel) or only the out-of-plane component (bottom panel) of the pumping field into account reveals that the direct excitation is exclusively caused by the out-of-plane pumping field.

only the in-plane component (top panel) or only the out-of-plane component (bottom panel) of the pumping field into account. In fact, this allows to disentangle the findings of Fig. S5(a), proving that the observed PP is exclusively caused by the in-plane pumping field as expected, while the forced excitation and the direct excitation are exclusively caused by the out-of-plane pumping field.
In contrast to the experimental results, a non-resonant pumping process populating the dipolar regime of the dispersion is not observed in these simulations. However, we would like to point out that the micro-magnetic simulations only include viscous Gilbert-type damping and are incapable to account for non-Gilbert type relaxation mechanisms, e.g., various magnon-phonon processes [4]. These processes can contribute significantly to the system's relaxation in high-quality YIG films, thus rendering the simulations unable to describe the real system. Still, an excitation of spin waves in the dipolar regime of the dispersion by the out-of-plane pumping field is observed here, but this mechanism can be excluded in the experiment, since the experimentally observed power law follows $m \neq 1$ as discussed in the following section.

## V. ASSOCIATED POWER LAW OF THE EXPERIMENTALLY OBSERVED PUMPING PROCESS

In Fig. S6, the order $m$ of the power law of the respective threshold curves of Fig. 2(c) of the manuscript is shown. The order is extracted from a linear fit of the threshold curve's rising slope (until saturation of the spin-wave population sets in) in a double-logarithmic plot of the measured intensity and the applied pumping power. A value $m \neq 1$ reveals that the underlying process is not a direct linear excitation process.

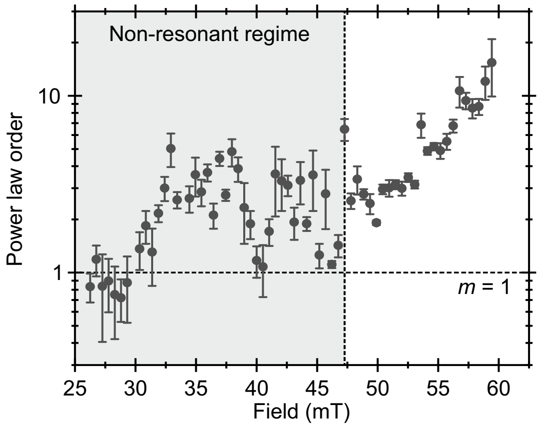


FIG. S6. Order $m$ of the associated power law ($Intensity \propto Power^m$) of the respective threshold curves of the 100 nm-wide conduit (Fig. 2(c) of the manuscript). Shaded area and vertical dashed black line mark the non-resonant pumping regime.

## VI. EXTRACTION OF THE EFFECTIVE SPIN-WAVE RELAXATION TIME

In Fig. S7(a), the approximation of the inverse spin-wave rise time according to Eq. 7 of the manuscript is exemplary shown for $\mu_0 H_{\text{ext}} = 55.4\,\text{mT}$. Figure S7(b) provides a comparison of the calculated theoretical relaxation time for the respective cases of pure Gilbert-type relaxation (bottom panel) and that the inhomogeneous linewidth broadening acts fully as a loss channel (top panel). The relaxation time is nearly constant within the investigated field range, since the spin-wave frequency is fixed to 3.5 GHz and the variation of the ellipticity coefficient is minor [see Fig. S1(b)].

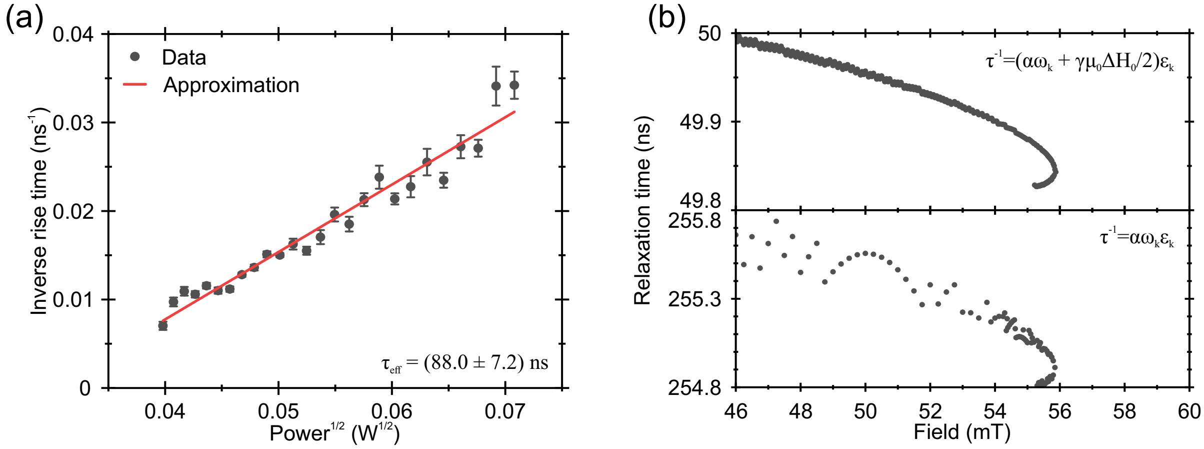


FIG. S7. (a) Exemplary approximation of the inverse spin-wave intensity rise time for $\mu_0 H_{\mathrm{ext}} = 55.4\,\mathrm{mT}$. (b) Calculated relaxation time for pure Gilbert-type relaxation (bottom panel) and included inhomogeneous linewidth broadening (top panel). Effective magnetization for the calculation: $M_{\mathrm{s}} = 115\,\mathrm{kAm}^{-1}$.

---


[1] Q. Wang, B. Heinz, R. Verba, M. Kewenig, P. Pirro, M. Schneider, T. Meyer, B. Lägel, C. Dubs, T. Brächer, and A. V. Chumak, Spin pinning and spin-wave dispersion in nanoscopic ferromagnetic waveguides, Phys. Rev. Lett. **122**, 247202 (2019).

[2] M. Mohseni, M. Kewenig, R. Verba, Q. Wang, M. Schneider, B. Heinz, F. Kohl, C. Dubs, B. Lägel, A. A. Serga, B. Hillebrands, A. V. Chumak, and P. Pirro, Parametric generation of propagating spin waves in ultrathin yttrium iron garnet waveguides, Phys. Status Solidi Rapid Res. Lett. **14**, 2070022 (2020).

[3] A. Vansteenkiste, J. Leliaert, M. Dvornik, M. Helsen, F. Garcia-Sanchez, and B. Van Waeyenberge, The design and verification of mumax3, AIP Adv. **4**, 107133 (2014).

[4] T. Kasuya and R. C. LeCraw, Relaxation mechanisms in ferromagnetic resonance, Phys. Rev. Lett. **6**, 223 (1961).
